# Supplementary material for: Render for CNN: Viewpoint Estimation in Images Using CNNs Trained with Rendered 3D Model Views
Source: arXiv:1505.05641 source file (2015-05-21)
Supplement: Supplementary file 1 [file supp_requirement.tex]

Authors may optionally upload supplementary material, which may not fit in the PDF size limit and may include:
videos to showcase results/demo of the proposed approach/system that were ready at the time of paper submission, but could not be included in the body of the paper due to reasons of format,
images, tables and other results that were ready at the time of paper submission, but could not be included in the body of the paper due to reasons of space,
anonymized related submissions to ICCV or other conferences and journals, and
appendices or technical reports containing extended proofs and mathematical derivations of results that are presented in the paper but could not be included due to reasons of space and are not essential to the understanding of the submitted paper.
ICCV encourages authors to submit videos using an MP4 codec such as DivX contained in an AVI. Also, please submit a README text file with each video specifying the exact codec used and a URL where the codec can be downloaded.

The authors should refer to the contents of the supplementary material appropriately in the paper. Note that reviewers will be encouraged to look at it, but are not obligated to do so. Please note that:

The paper for review (PDF only) must be submitted first before the supplementary material (PDF or ZIP only) can be submitted.
All supplementary material must be self-contained and zipped into a single file. The following formats are allowed: avi, doc, docx, mp4, pdf, wmv. CMT imposes a 100MB limit on the size of this file. Note that you can update the file by uploading a new one (the old one will be deleted and replaced).
Please make sure that the supplementary material directly supports the paper as submitted prior to the paper deadline. ONLY results generated by the algorithm/approach/system reported in the submitted version are allowed. Material based on improvements subsequent to the paper deadline is not allowed. In particular, new experiments on new datasets, new experiments on the same datasets obtained by using new parameters or by re-training the model are NOT allowed.
Do not submit a newer version of the paper as supplementary material. A newer version of the paper or portion thereof, with description of an improved algorithm/approach/system or even one spelling or typo correction, is not allowed.
